# Supplementary material for: AppMine: Behavioral Analytics for Web Application Vulnerability Detection
Source: arXiv:1908.01928 source file (2019-08-06)
Supplement: Supplementary file 1 [file appendix.tex]

\appendix

%\subsection{List of post-exploit (attack) scripts}

%sample text

%\cleardoublepage

\section{ROC curves for attacks}

\begin{figure*}[h]
\centering
\begin{subfigure}{0.3\textwidth}
	\centering
	\includegraphics[height=0.15\textheight,keepaspectratio]{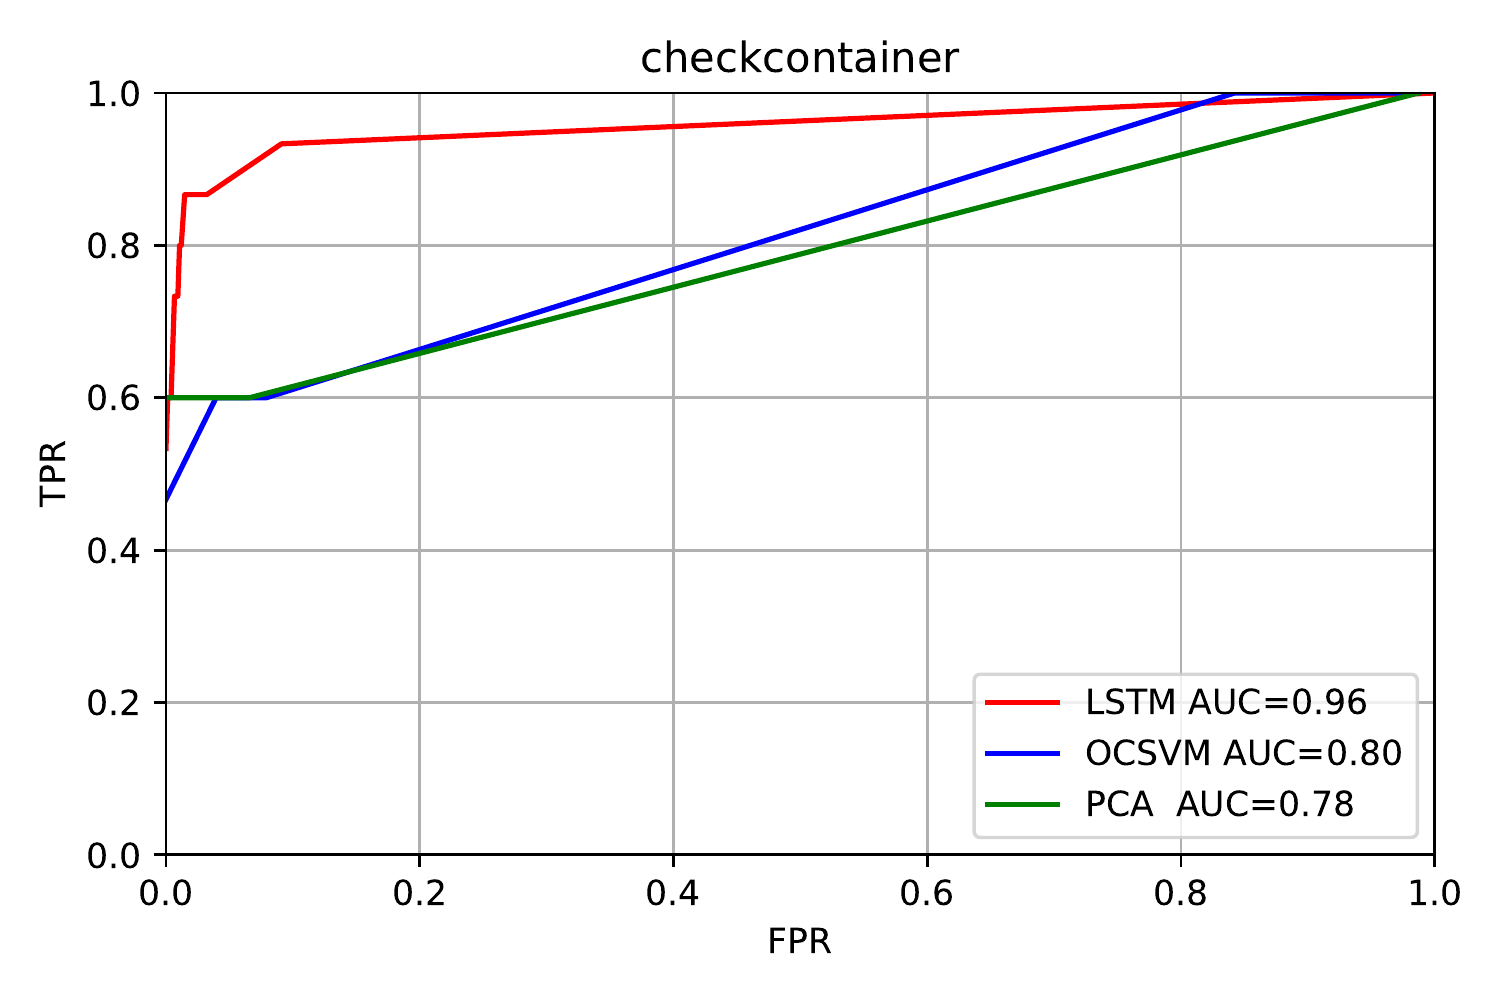}
	%\caption{Drupal}
	%\label{fig:drupal_allrocs}
\end{subfigure}
\hfill
\begin{subfigure}{0.3\textwidth}
         \centering
         \includegraphics[height=0.15\textheight,keepaspectratio]{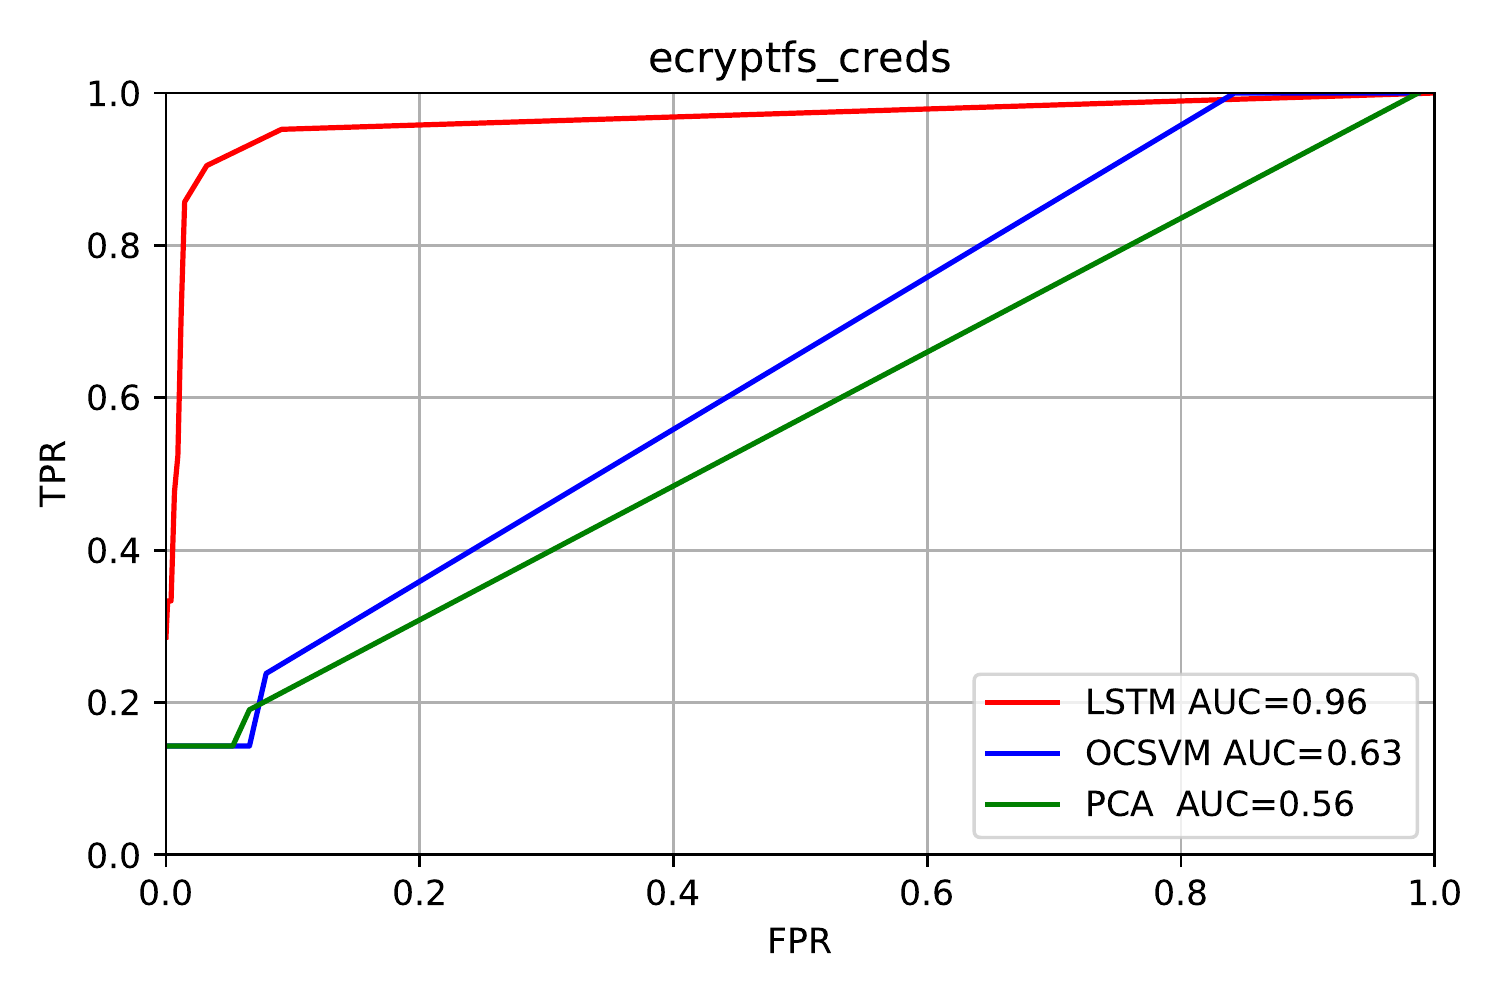}
         %\caption{ProFTPD}
         %\label{fig:proftpd_allrocs}
\end{subfigure}
\hfill
\begin{subfigure}{0.3\textwidth}
        \centering
         \includegraphics[height=0.15\textheight,keepaspectratio]{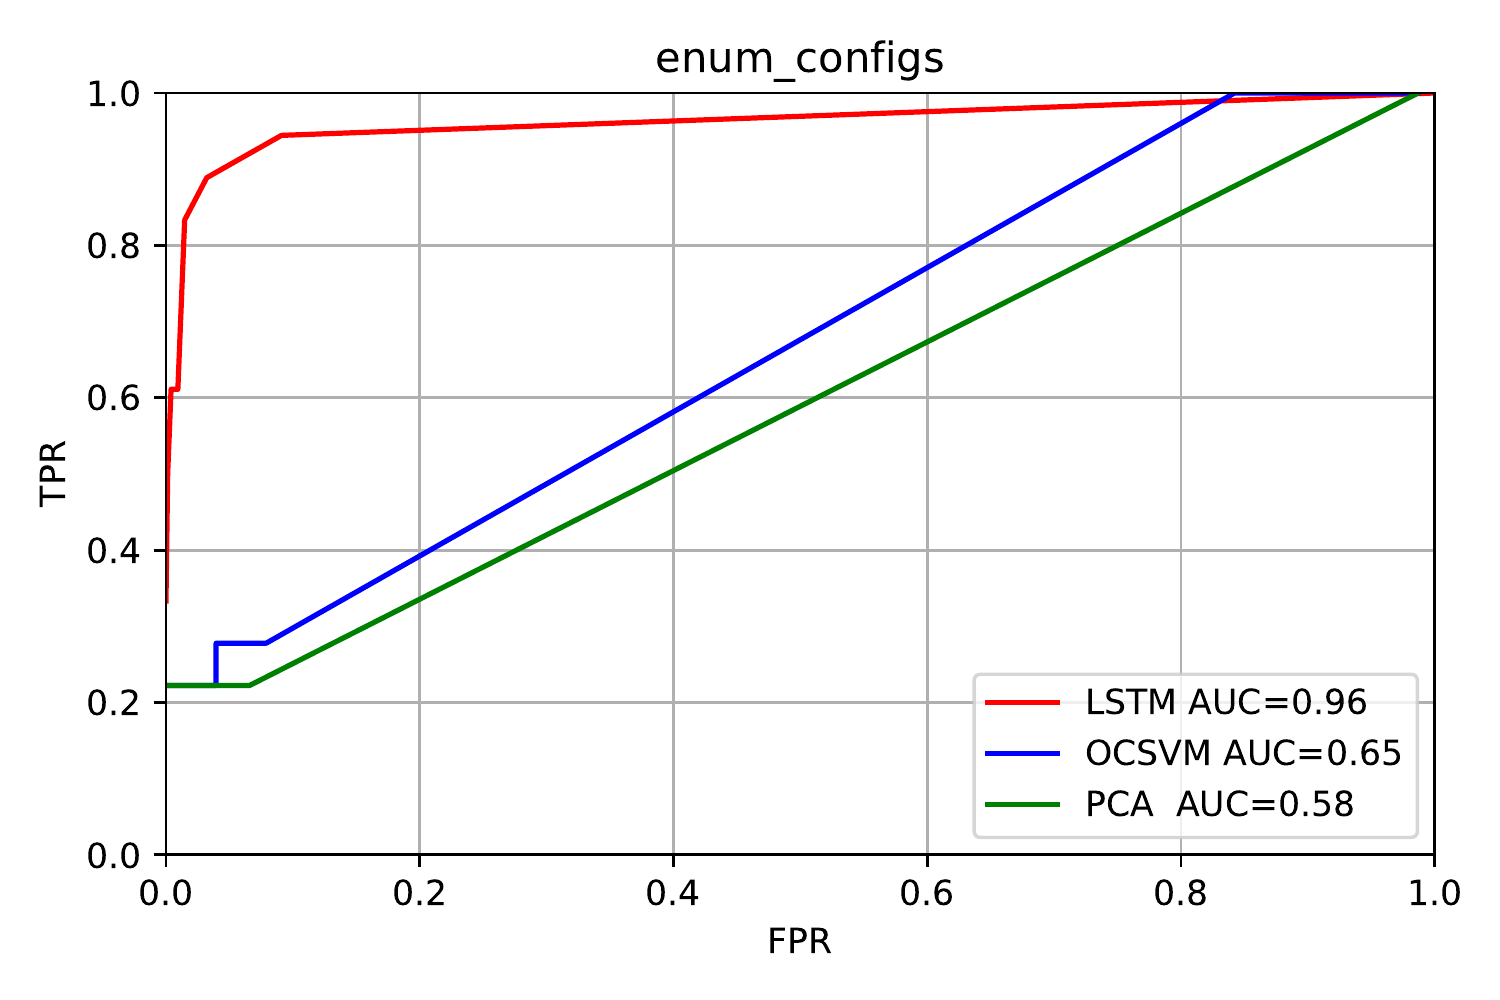}
         %\caption{Struts CVE-207-5638}
         %\label{fig:struts5638_allrocs}
\end{subfigure}

\smallskip
\begin{subfigure}{0.3\textwidth}
	\centering
	\includegraphics[height=0.15\textheight,keepaspectratio]{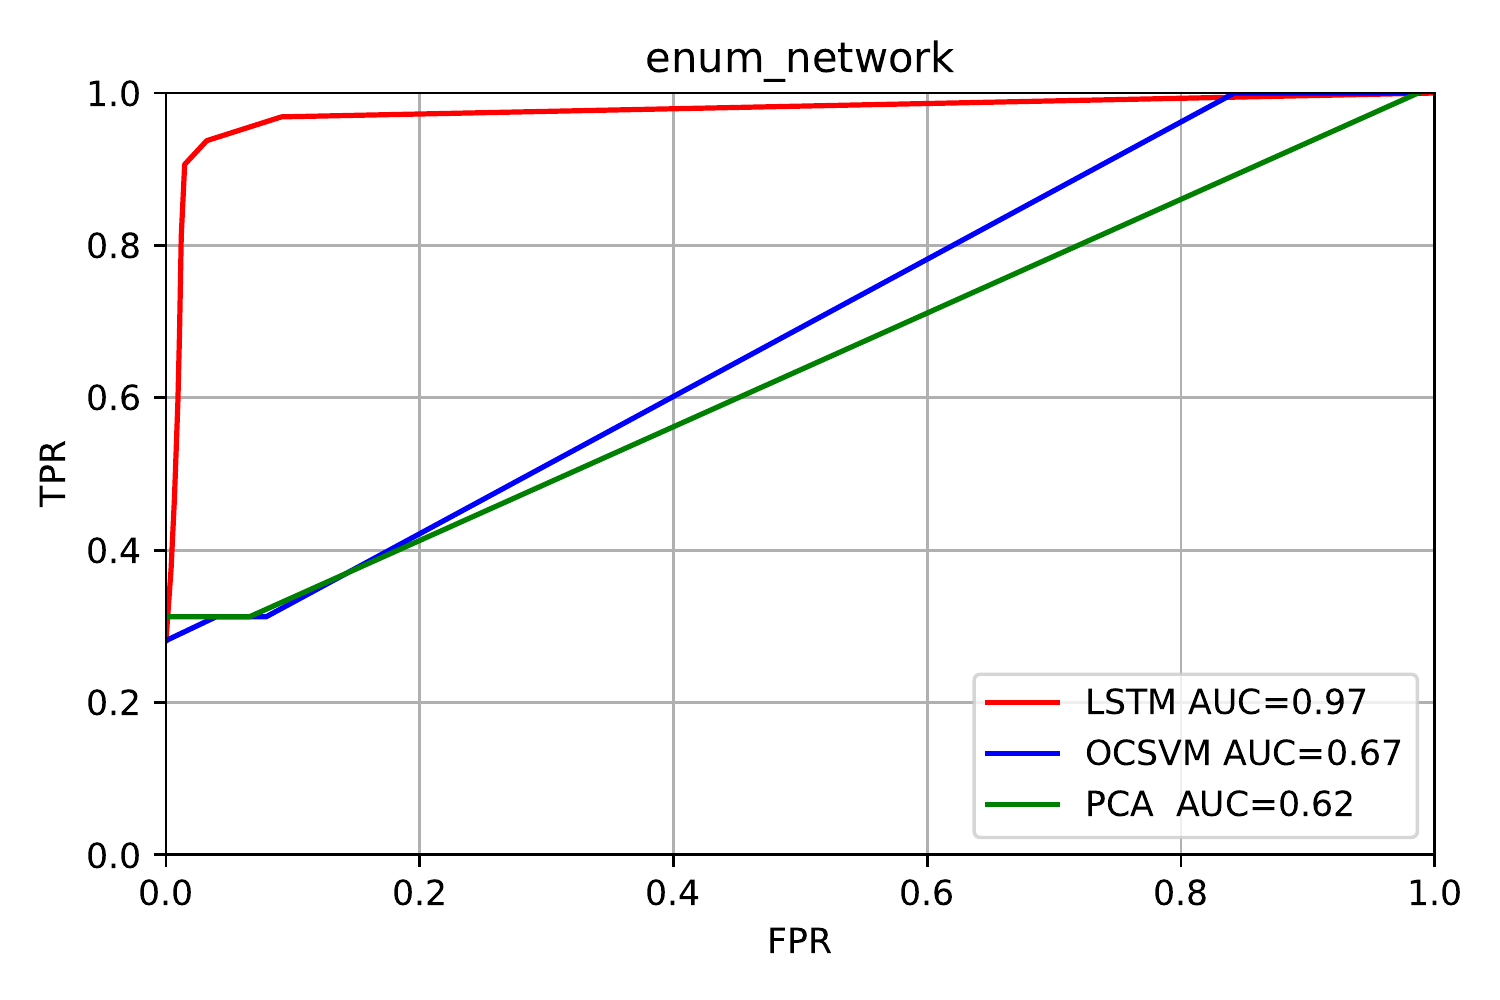}
	%\caption{Drupal}
	%\label{fig:drupal_allrocs}
\end{subfigure}
\hfill
\begin{subfigure}{0.3\textwidth}
         \centering
         \includegraphics[height=0.15\textheight,keepaspectratio]{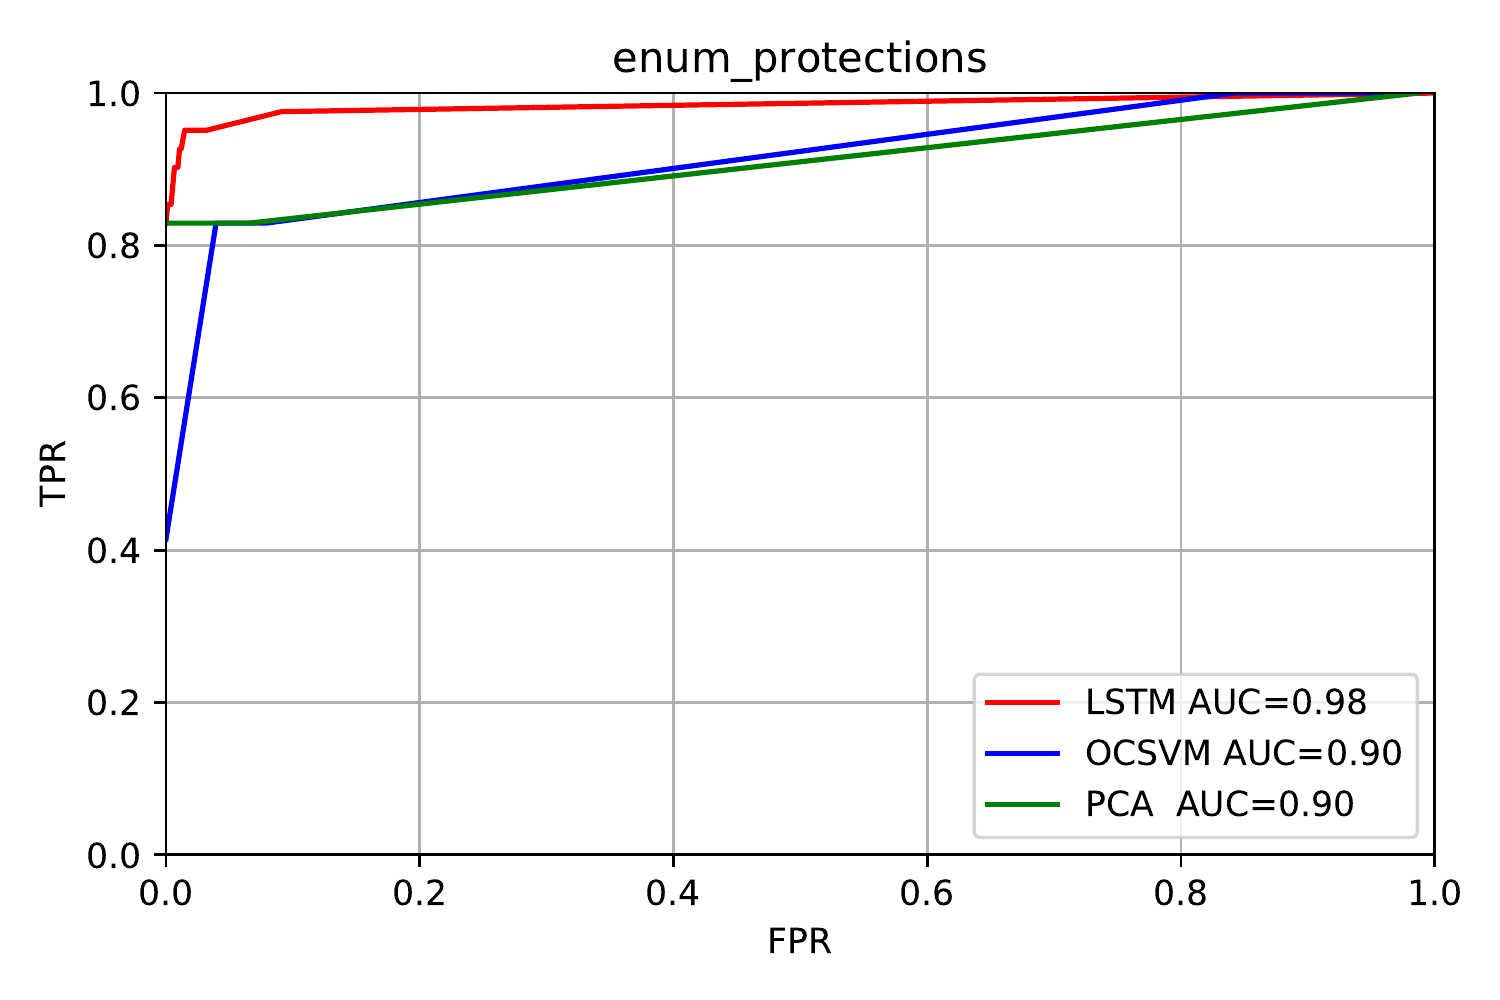}
         %\caption{ProFTPD}
         %\label{fig:proftpd_allrocs}
\end{subfigure}
\hfill
\begin{subfigure}{0.3\textwidth}
        \centering
         \includegraphics[height=0.15\textheight,keepaspectratio]{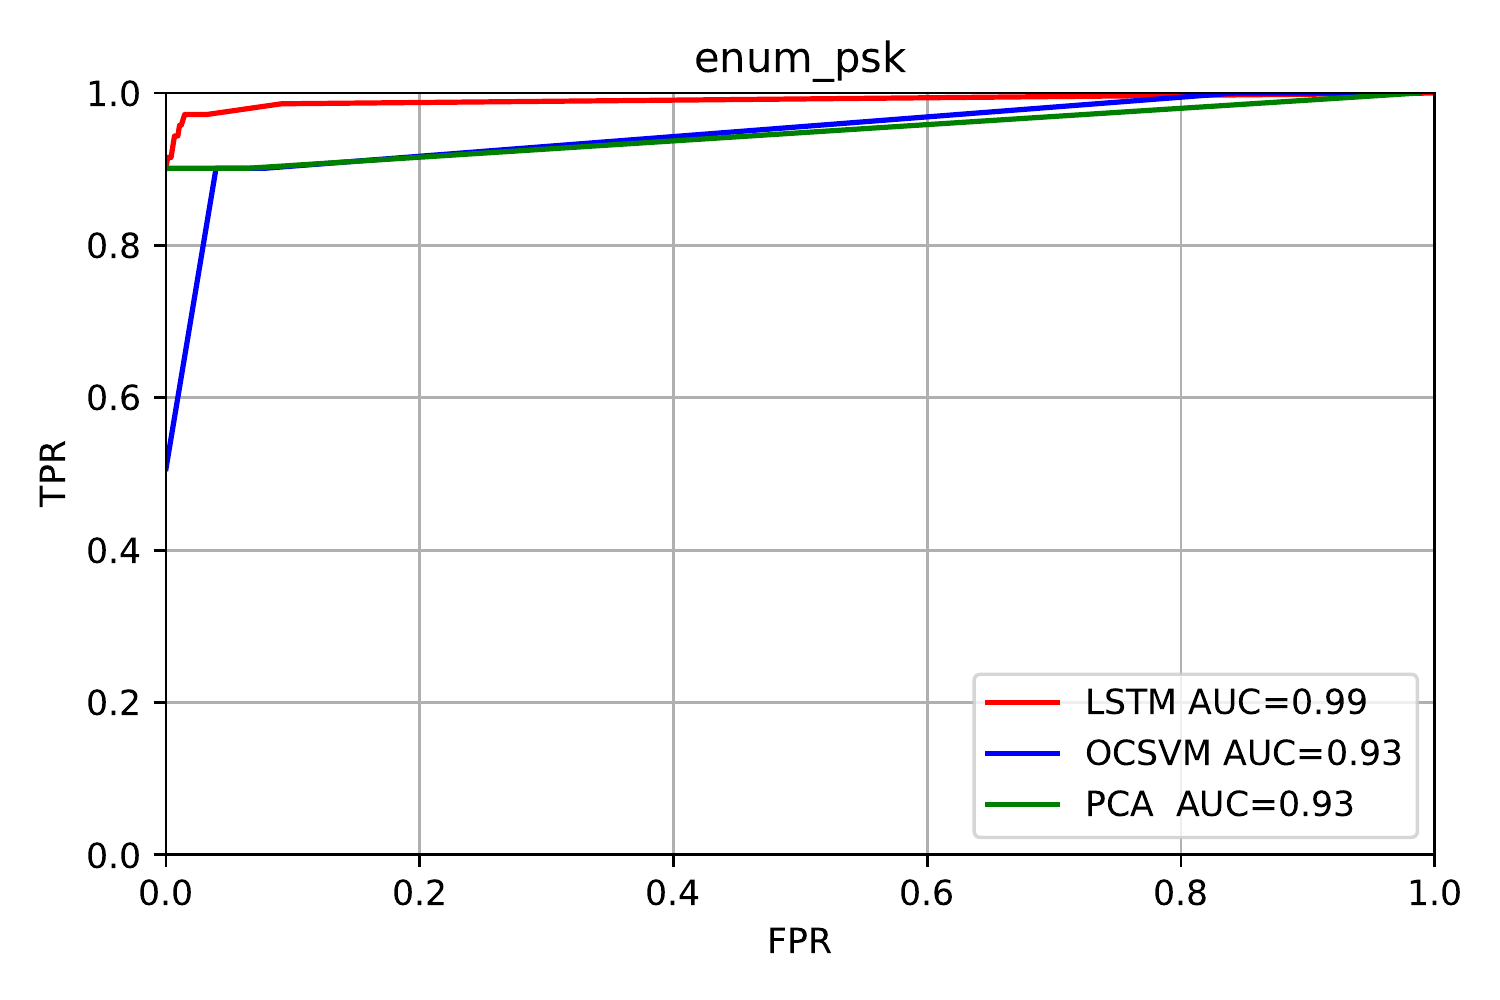}
         %\caption{Struts CVE-207-5638}
         %\label{fig:struts5638_allrocs}
\end{subfigure}

\smallskip
\begin{subfigure}{0.3\textwidth}
	\centering
	\includegraphics[height=0.15\textheight,keepaspectratio]{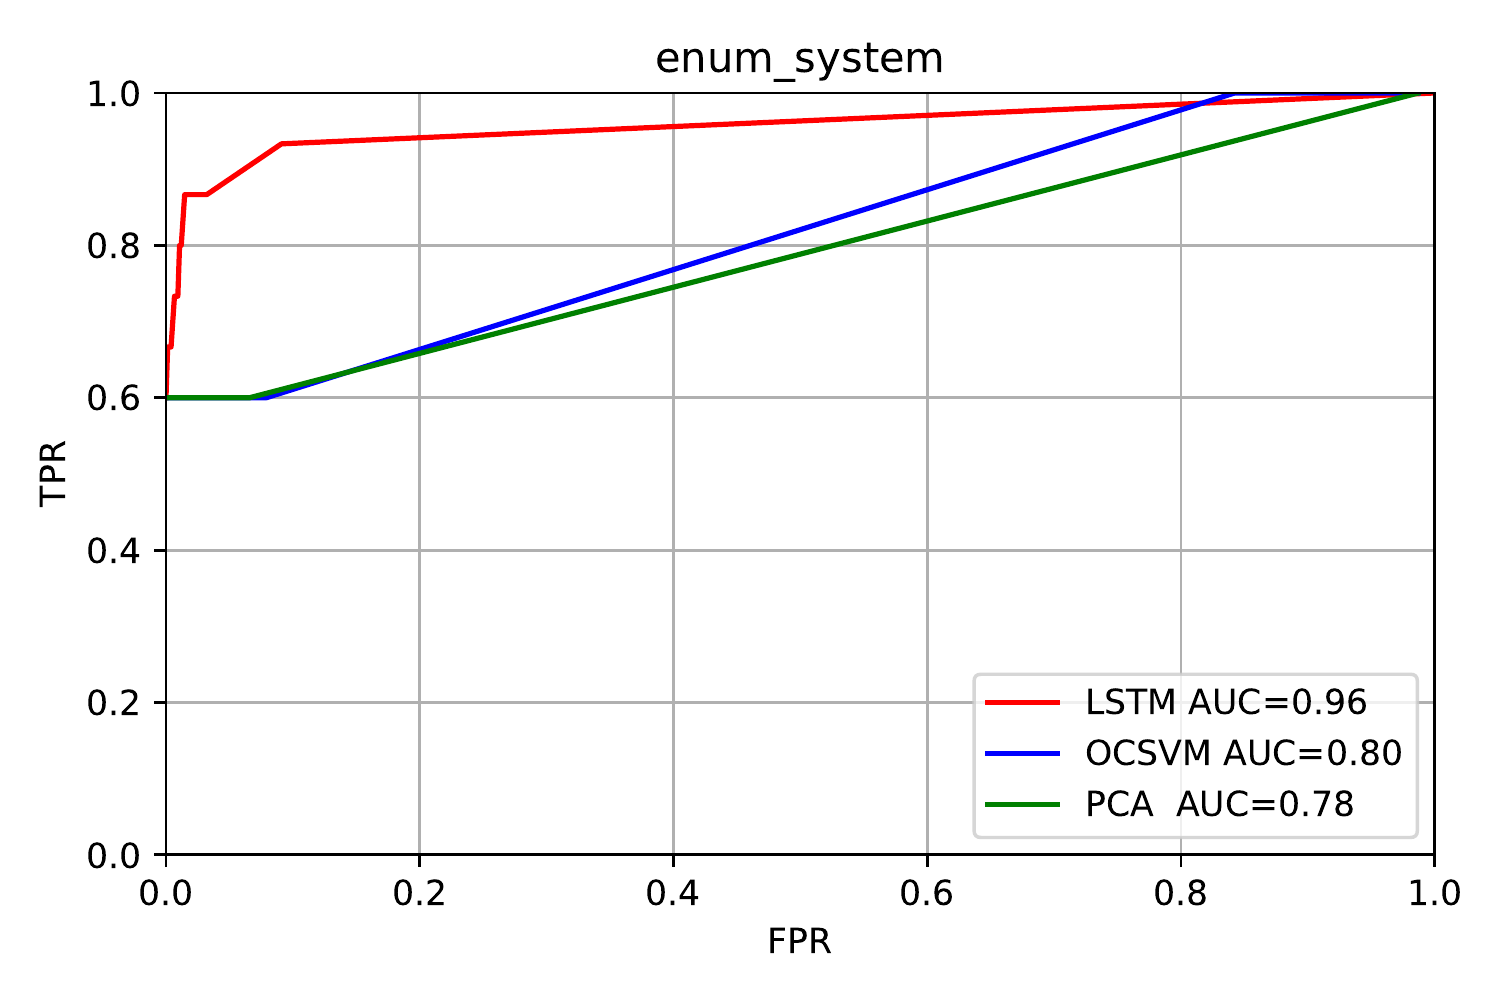}
	%\caption{Drupal}
	%\label{fig:drupal_allrocs}
\end{subfigure}
\hfill
\begin{subfigure}{0.3\textwidth}
         \centering
         \includegraphics[height=0.15\textheight,keepaspectratio]{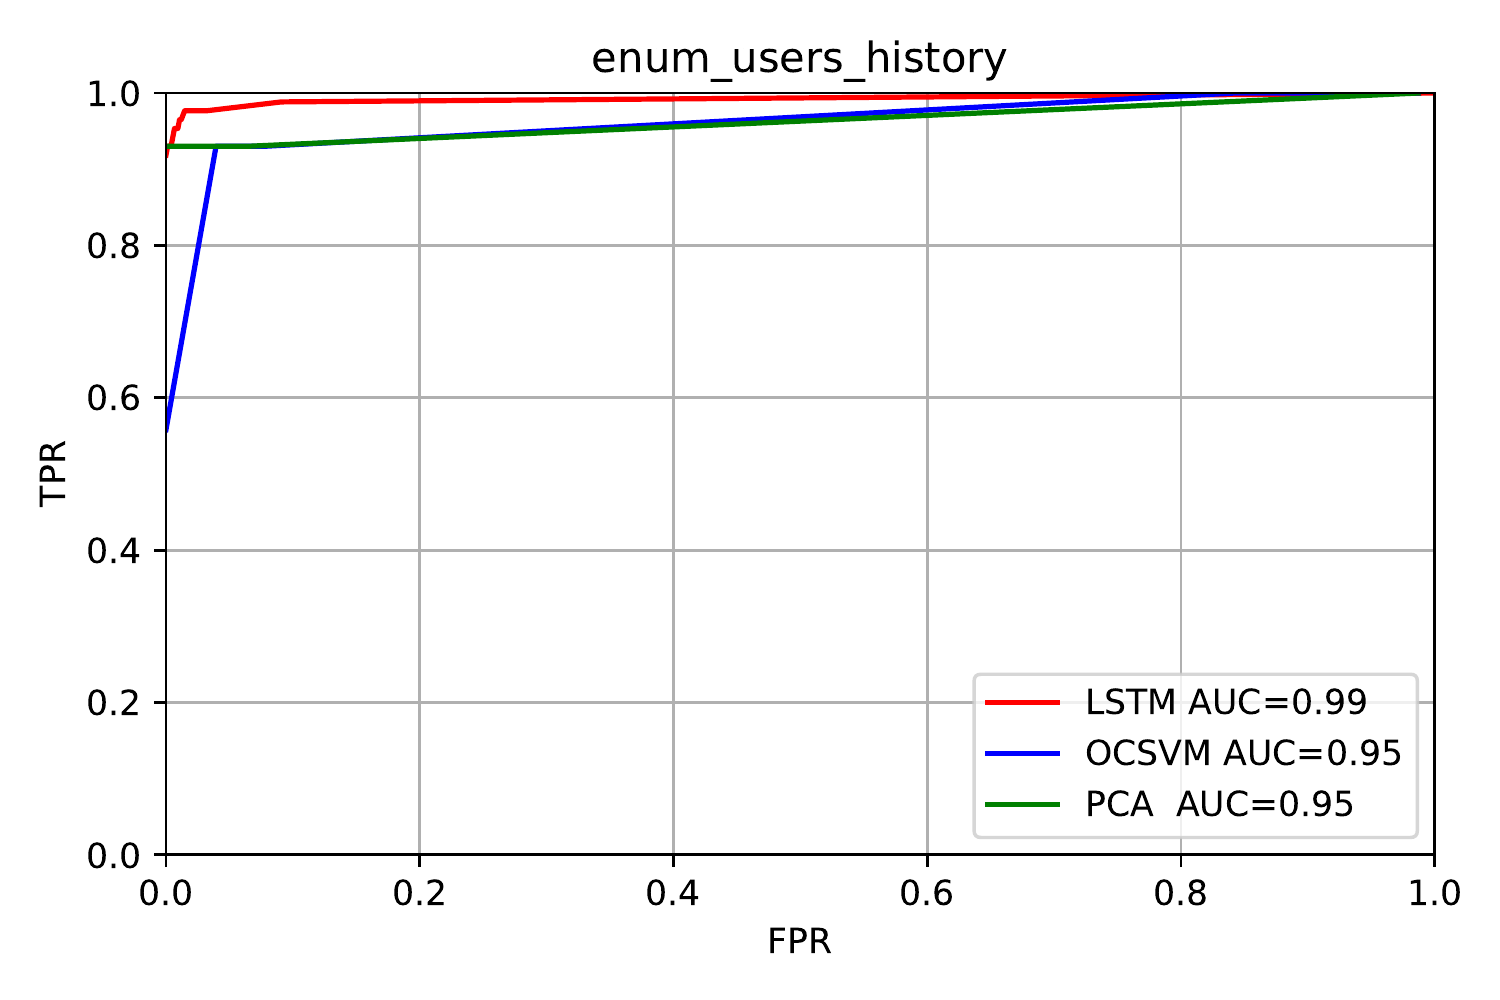}
         %\caption{ProFTPD}
         %\label{fig:proftpd_allrocs}
\end{subfigure}
\hfill
\begin{subfigure}{0.3\textwidth}
        \centering
         \includegraphics[height=0.15\textheight,keepaspectratio]{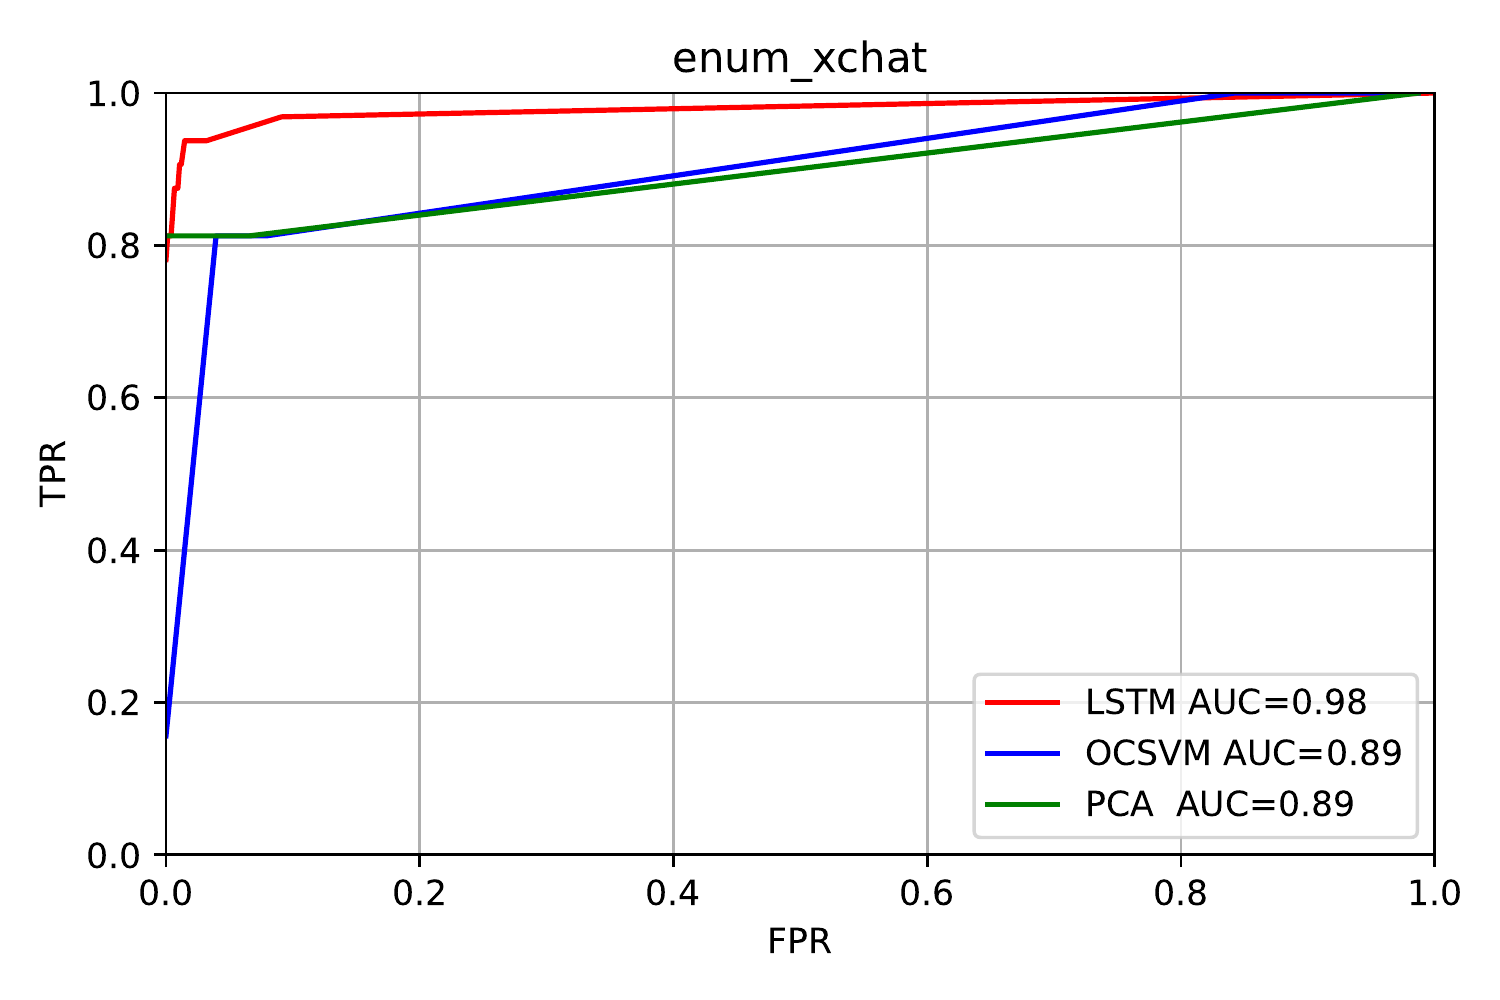}
         %\caption{Struts CVE-207-5638}
         %\label{fig:struts5638_allrocs}
\end{subfigure}

\smallskip
\begin{subfigure}{0.3\textwidth}
	\centering
	\includegraphics[height=0.15\textheight,keepaspectratio]{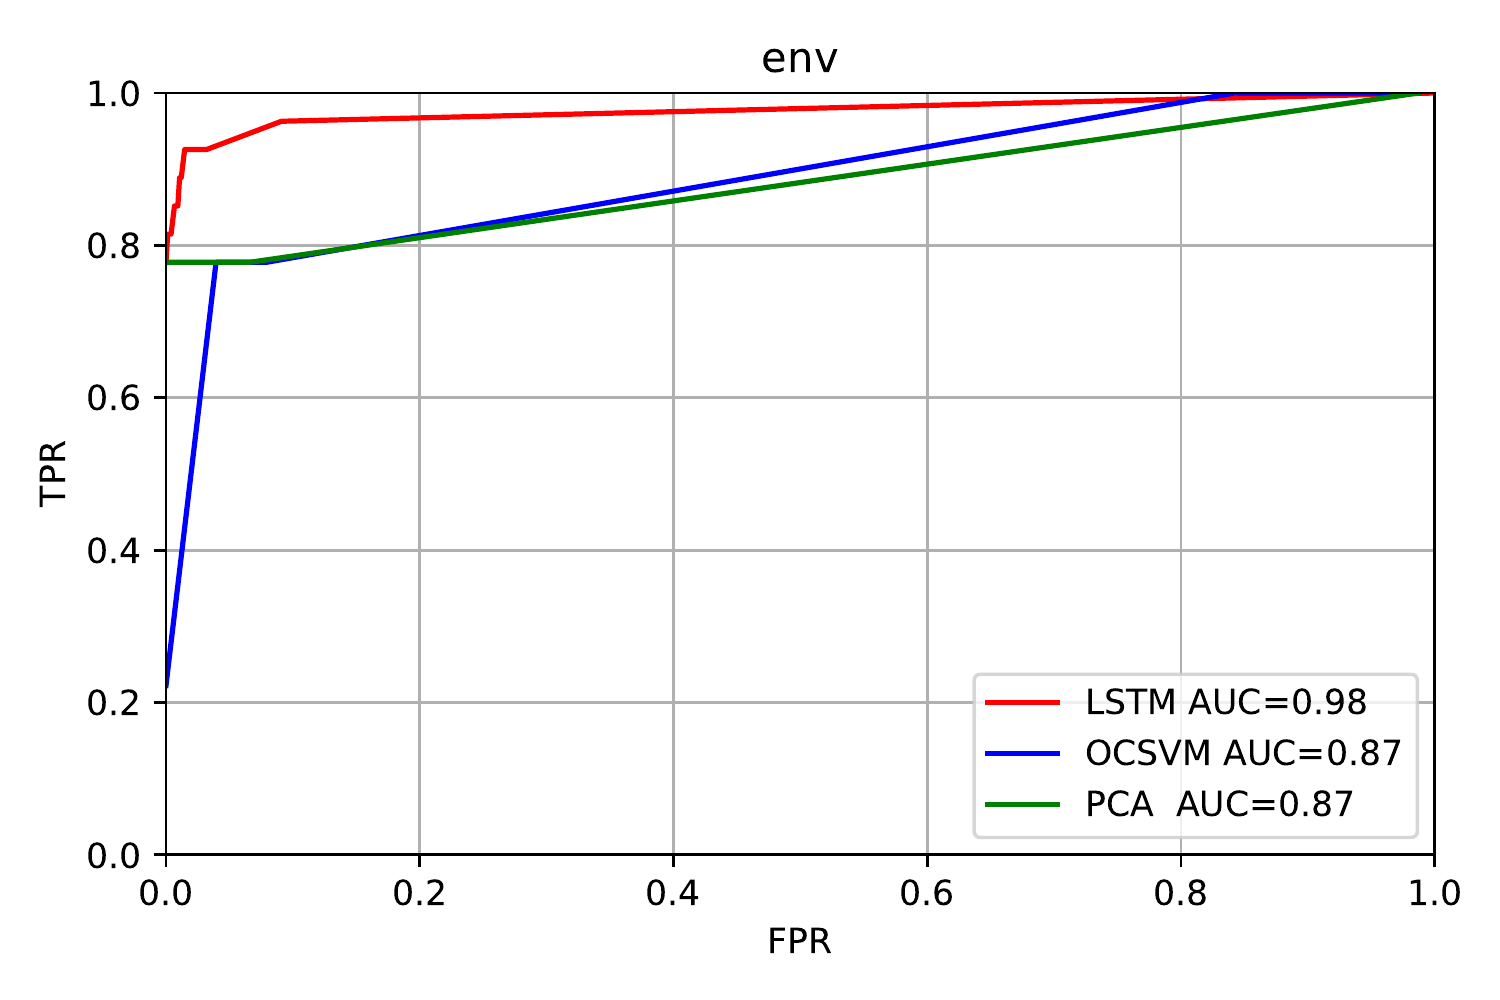}
	%\caption{Drupal}
	%\label{fig:drupal_allrocs}
\end{subfigure}
\hfill
\begin{subfigure}{0.3\textwidth}
         \centering
         \includegraphics[height=0.15\textheight,keepaspectratio]{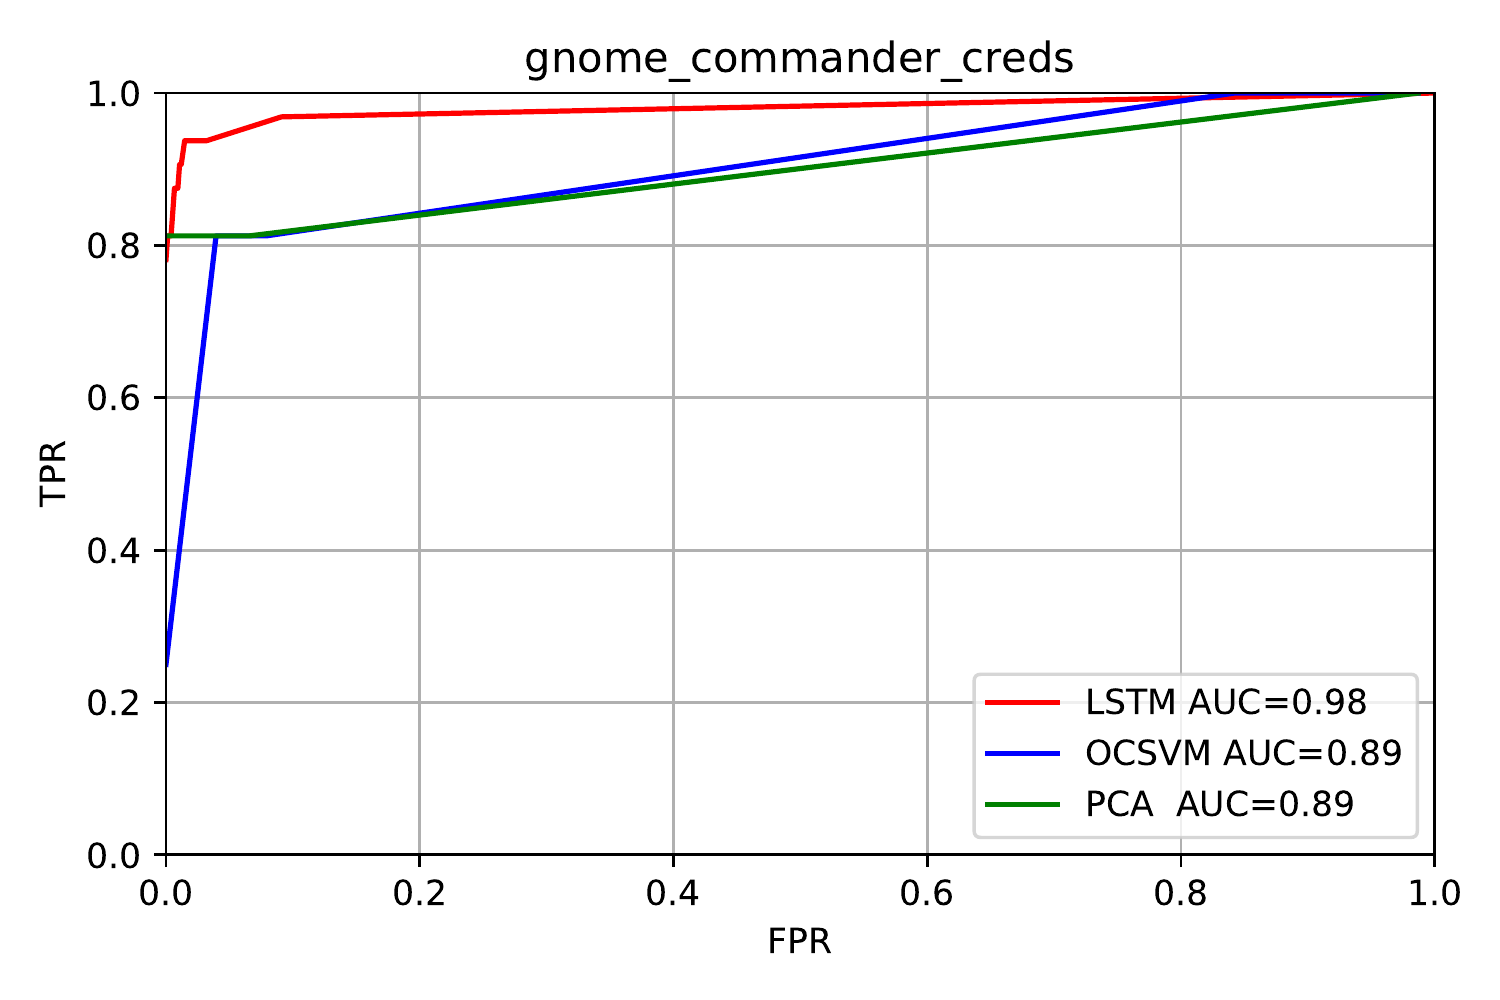}
         %\caption{ProFTPD}
         %\label{fig:proftpd_allrocs}
\end{subfigure}
\hfill
\begin{subfigure}{0.3\textwidth}
        \centering
         \includegraphics[height=0.15\textheight,keepaspectratio]{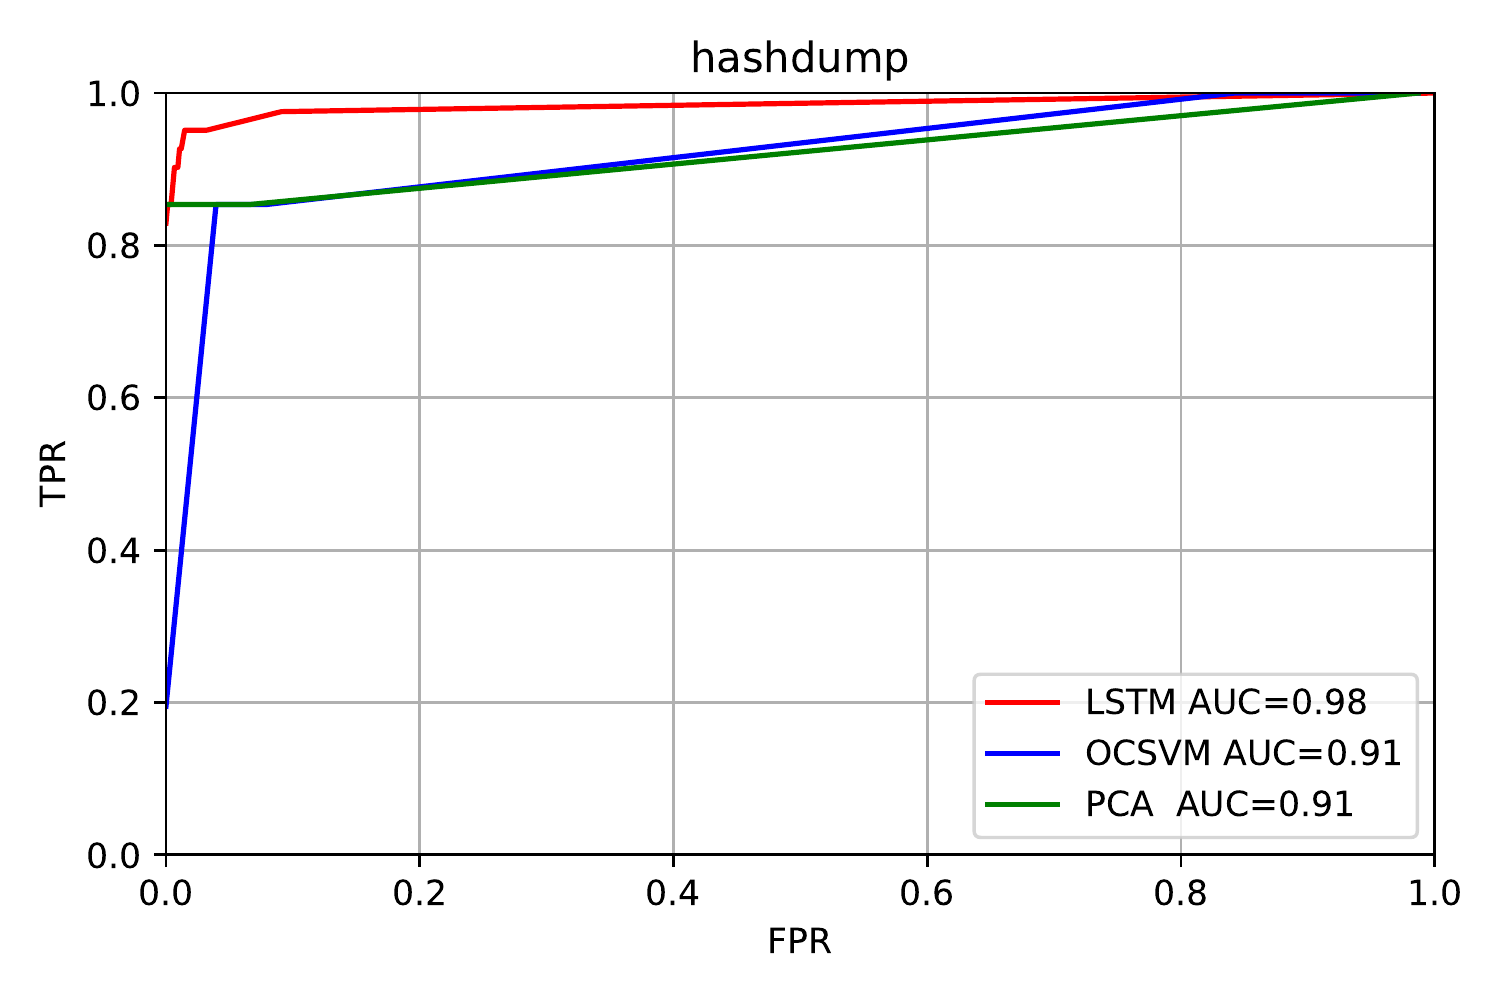}
         %\caption{Struts CVE-207-5638}
         %\label{fig:struts5638_allrocs}
\end{subfigure}

\smallskip
\begin{subfigure}{0.3\textwidth}
	\centering
	\includegraphics[height=0.15\textheight,keepaspectratio]{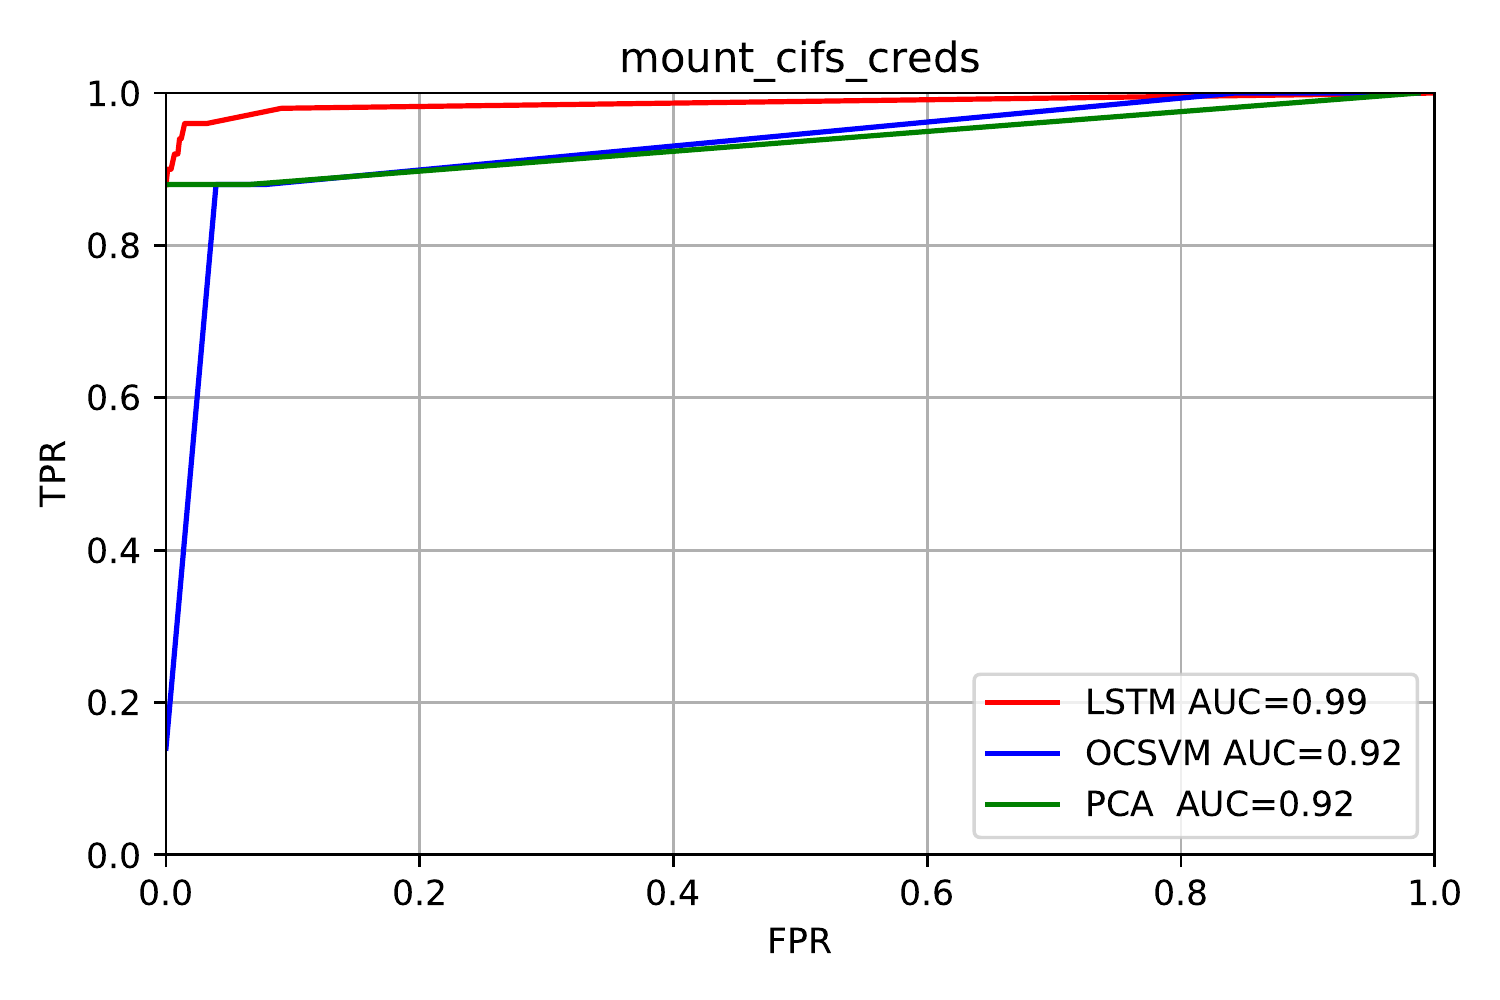}
	%\caption{Drupal}
	%\label{fig:drupal_allrocs}
\end{subfigure}
\hfill
\begin{subfigure}{0.3\textwidth}
         \centering
         \includegraphics[height=0.15\textheight,keepaspectratio]{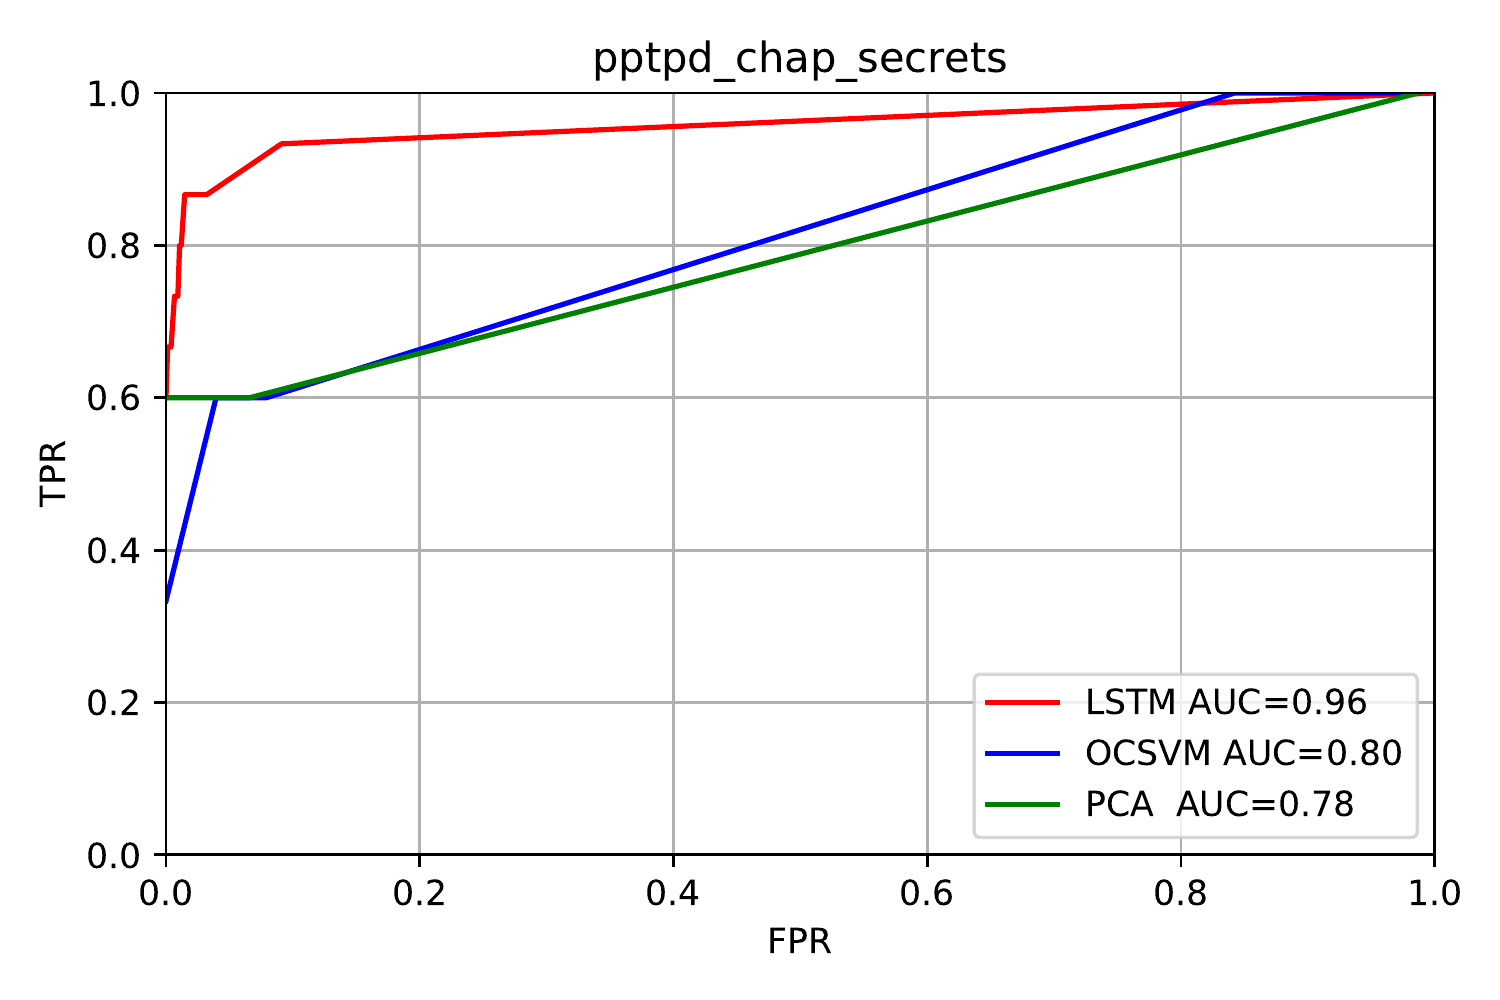}
         %\caption{ProFTPD}
         %\label{fig:proftpd_allrocs}
\end{subfigure}
\hfill
\begin{subfigure}{0.3\textwidth}
        \centering
         \includegraphics[height=0.15\textheight,keepaspectratio]{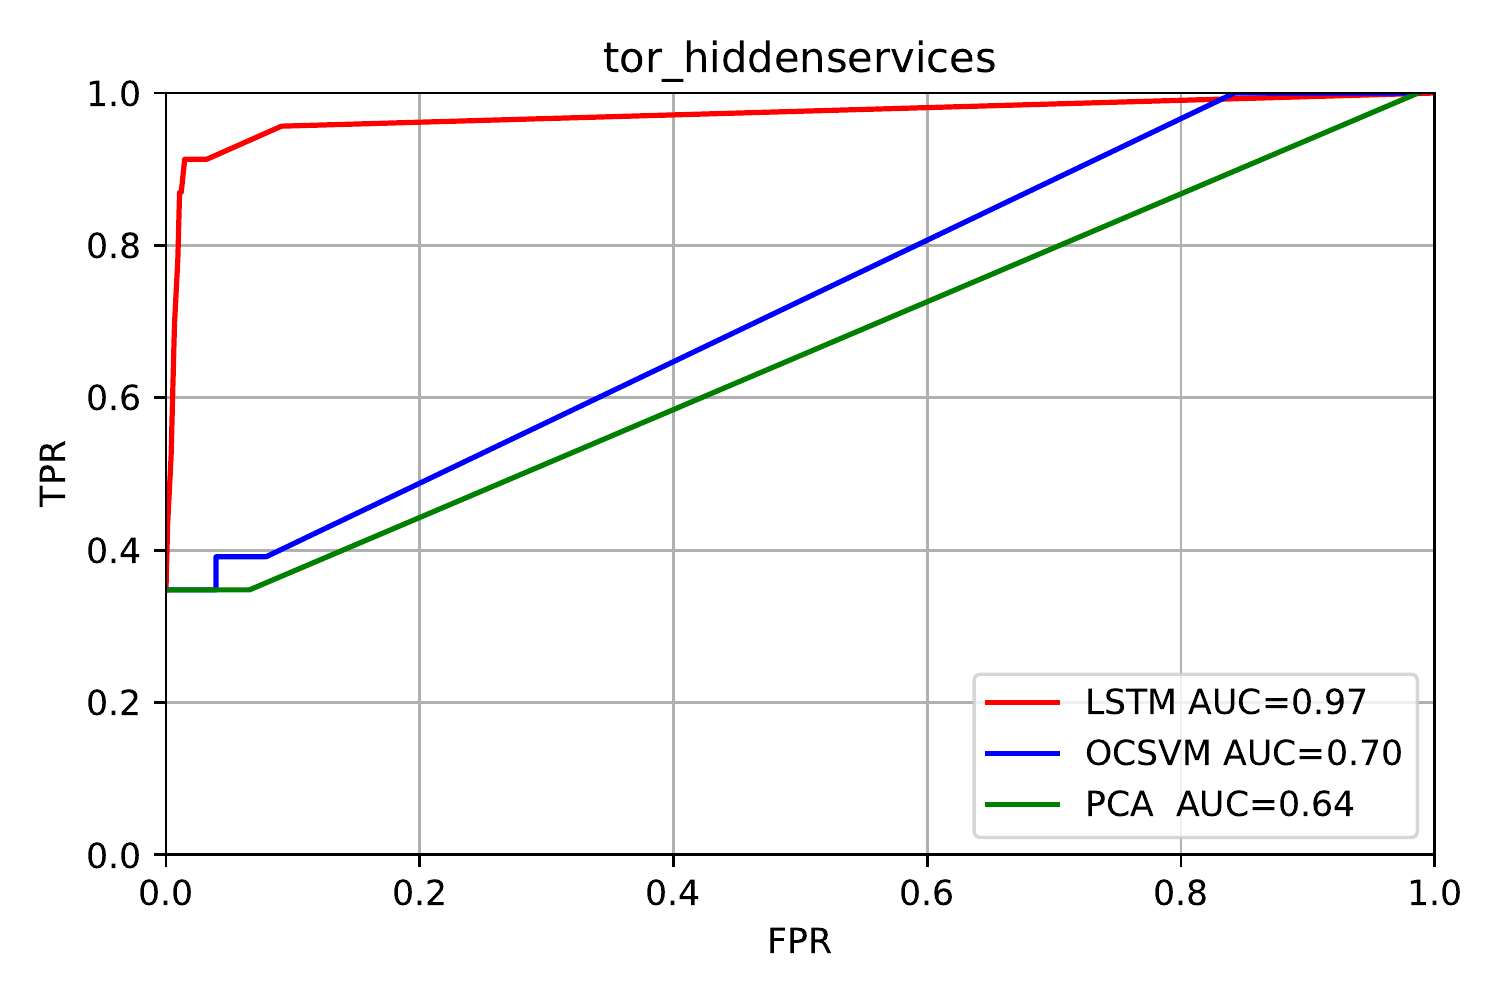}
         %\caption{Struts CVE-207-5638}
         %\label{fig:struts5638_allrocs}
\end{subfigure}
\caption{ROC curves for attack scripts for Struts CVE-2017-5638}
%\label{fig:allrocs}
\end{figure*}

\begin{figure*}[h]
\centering
\begin{subfigure}{0.3\textwidth}
	\centering
	\includegraphics[height=0.15\textheight,keepaspectratio]{Figures/struts9805combined/struts9805_combined_checkcontainer.pdf}
	%\caption{Drupal}
	%\label{fig:drupal_allrocs}
\end{subfigure}
\hfill
\begin{subfigure}{0.3\textwidth}
         \centering
         \includegraphics[height=0.15\textheight,keepaspectratio]{Figures/struts9805combined/struts9805_combined_ecryptfs_creds.pdf}
         %\caption{ProFTPD}
         %\label{fig:proftpd_allrocs}
\end{subfigure}
\hfill
\begin{subfigure}{0.3\textwidth}
        \centering
         \includegraphics[height=0.15\textheight,keepaspectratio]{Figures/struts9805combined/struts9805_combined_enum_configs.pdf}
         %\caption{Struts CVE-207-5638}
         %\label{fig:struts9805_allrocs}
\end{subfigure}

\smallskip
\begin{subfigure}{0.3\textwidth}
	\centering
	\includegraphics[height=0.15\textheight,keepaspectratio]{Figures/struts9805combined/struts9805_combined_enum_network.pdf}
	%\caption{Drupal}
	%\label{fig:drupal_allrocs}
\end{subfigure}
\hfill
\begin{subfigure}{0.3\textwidth}
         \centering
         \includegraphics[height=0.15\textheight,keepaspectratio]{Figures/struts9805combined/struts9805_combined_enum_protections.pdf}
         %\caption{ProFTPD}
         %\label{fig:proftpd_allrocs}
\end{subfigure}
\hfill
\begin{subfigure}{0.3\textwidth}
        \centering
         \includegraphics[height=0.15\textheight,keepaspectratio]{Figures/struts9805combined/struts9805_combined_enum_psk.pdf}
         %\caption{Struts CVE-207-5638}
         %\label{fig:struts9805_allrocs}
\end{subfigure}

\smallskip
\begin{subfigure}{0.3\textwidth}
	\centering
	\includegraphics[height=0.15\textheight,keepaspectratio]{Figures/struts9805combined/struts9805_combined_enum_system.pdf}
	%\caption{Drupal}
	%\label{fig:drupal_allrocs}
\end{subfigure}
\hfill
\begin{subfigure}{0.3\textwidth}
         \centering
         \includegraphics[height=0.15\textheight,keepaspectratio]{Figures/struts9805combined/struts9805_combined_enum_users_history.pdf}
         %\caption{ProFTPD}
         %\label{fig:proftpd_allrocs}
\end{subfigure}
\hfill
\begin{subfigure}{0.3\textwidth}
        \centering
         \includegraphics[height=0.15\textheight,keepaspectratio]{Figures/struts9805combined/struts9805_combined_enum_xchat.pdf}
         %\caption{Struts CVE-207-5638}
         %\label{fig:struts9805_allrocs}
\end{subfigure}

\smallskip
\begin{subfigure}{0.3\textwidth}
	\centering
	\includegraphics[height=0.15\textheight,keepaspectratio]{Figures/struts9805combined/struts9805_combined_env.pdf}
	%\caption{Drupal}
	%\label{fig:drupal_allrocs}
\end{subfigure}
\hfill
\begin{subfigure}{0.3\textwidth}
         \centering
         \includegraphics[height=0.15\textheight,keepaspectratio]{Figures/struts9805combined/struts9805_combined_gnome_commander_creds.pdf}
         %\caption{ProFTPD}
         %\label{fig:proftpd_allrocs}
\end{subfigure}
\hfill
\begin{subfigure}{0.3\textwidth}
        \centering
         \includegraphics[height=0.15\textheight,keepaspectratio]{Figures/struts9805combined/struts9805_combined_hashdump.pdf}
         %\caption{Struts CVE-207-5638}
         %\label{fig:struts9805_allrocs}
\end{subfigure}

\smallskip
\begin{subfigure}{0.3\textwidth}
	\centering
	\includegraphics[height=0.15\textheight,keepaspectratio]{Figures/struts9805combined/struts9805_combined_mount_cifs_creds.pdf}
	%\caption{Drupal}
	%\label{fig:drupal_allrocs}
\end{subfigure}
\hfill
\begin{subfigure}{0.3\textwidth}
         \centering
         \includegraphics[height=0.15\textheight,keepaspectratio]{Figures/struts9805combined/struts9805_combined_pptpd_chap_secrets.pdf}
         %\caption{ProFTPD}
         %\label{fig:proftpd_allrocs}
\end{subfigure}
\hfill
\begin{subfigure}{0.3\textwidth}
        \centering
         \includegraphics[height=0.15\textheight,keepaspectratio]{Figures/struts9805combined/struts9805_combined_tor_hiddenservices.pdf}
         %\caption{Struts CVE-207-5638}
         %\label{fig:struts9805_allrocs}
\end{subfigure}
\caption{ROC curves for attack scripts for Struts CVE-2017-9805}
%\label{fig:allrocs}
\end{figure*}

\begin{figure*}[h]
\centering
\begin{subfigure}{0.3\textwidth}
	\centering
	\includegraphics[height=0.15\textheight,keepaspectratio]{Figures/drupalcombined/drupal_combined_checkcontainer.pdf}
	%\caption{Drupal}
	%\label{fig:drupal_allrocs}
\end{subfigure}
\hfill
\begin{subfigure}{0.3\textwidth}
         \centering
         \includegraphics[height=0.15\textheight,keepaspectratio]{Figures/drupalcombined/drupal_combined_ecryptfs_creds.pdf}
         %\caption{ProFTPD}
         %\label{fig:proftpd_allrocs}
\end{subfigure}
\hfill
\begin{subfigure}{0.3\textwidth}
        \centering
         \includegraphics[height=0.15\textheight,keepaspectratio]{Figures/drupalcombined/drupal_combined_enum_configs.pdf}
         %\caption{Struts CVE-207-5638}
         %\label{fig:drupal_allrocs}
\end{subfigure}

\smallskip
\begin{subfigure}{0.3\textwidth}
	\centering
	\includegraphics[height=0.15\textheight,keepaspectratio]{Figures/drupalcombined/drupal_combined_enum_network.pdf}
	%\caption{Drupal}
	%\label{fig:drupal_allrocs}
\end{subfigure}
\hfill
\begin{subfigure}{0.3\textwidth}
         \centering
         \includegraphics[height=0.15\textheight,keepaspectratio]{Figures/drupalcombined/drupal_combined_enum_protections.pdf}
         %\caption{ProFTPD}
         %\label{fig:proftpd_allrocs}
\end{subfigure}
\hfill
\begin{subfigure}{0.3\textwidth}
        \centering
         \includegraphics[height=0.15\textheight,keepaspectratio]{Figures/drupalcombined/drupal_combined_enum_psk.pdf}
         %\caption{Struts CVE-207-5638}
         %\label{fig:drupal_allrocs}
\end{subfigure}

\smallskip
\begin{subfigure}{0.3\textwidth}
	\centering
	\includegraphics[height=0.15\textheight,keepaspectratio]{Figures/drupalcombined/drupal_combined_enum_system.pdf}
	%\caption{Drupal}
	%\label{fig:drupal_allrocs}
\end{subfigure}
\hfill
\begin{subfigure}{0.3\textwidth}
         \centering
         \includegraphics[height=0.15\textheight,keepaspectratio]{Figures/drupalcombined/drupal_combined_enum_users_history.pdf}
         %\caption{ProFTPD}
         %\label{fig:proftpd_allrocs}
\end{subfigure}
\hfill
\begin{subfigure}{0.3\textwidth}
        \centering
         \includegraphics[height=0.15\textheight,keepaspectratio]{Figures/drupalcombined/drupal_combined_enum_xchat.pdf}
         %\caption{Struts CVE-207-5638}
         %\label{fig:drupal_allrocs}
\end{subfigure}

\smallskip
\begin{subfigure}{0.3\textwidth}
	\centering
	\includegraphics[height=0.15\textheight,keepaspectratio]{Figures/drupalcombined/drupal_combined_env.pdf}
	%\caption{Drupal}
	%\label{fig:drupal_allrocs}
\end{subfigure}
\hfill
\begin{subfigure}{0.3\textwidth}
         \centering
         \includegraphics[height=0.15\textheight,keepaspectratio]{Figures/drupalcombined/drupal_combined_gnome_commander_creds.pdf}
         %\caption{ProFTPD}
         %\label{fig:proftpd_allrocs}
\end{subfigure}
\hfill
\begin{subfigure}{0.3\textwidth}
        \centering
         \includegraphics[height=0.15\textheight,keepaspectratio]{Figures/drupalcombined/drupal_combined_hashdump.pdf}
         %\caption{Struts CVE-207-5638}
         %\label{fig:drupal_allrocs}
\end{subfigure}

\smallskip
\begin{subfigure}{0.3\textwidth}
	\centering
	\includegraphics[height=0.15\textheight,keepaspectratio]{Figures/drupalcombined/drupal_combined_mount_cifs_creds.pdf}
	%\caption{Drupal}
	%\label{fig:drupal_allrocs}
\end{subfigure}
\hfill
\begin{subfigure}{0.3\textwidth}
         \centering
         \includegraphics[height=0.15\textheight,keepaspectratio]{Figures/drupalcombined/drupal_combined_pptpd_chap_secrets.pdf}
         %\caption{ProFTPD}
         %\label{fig:proftpd_allrocs}
\end{subfigure}
\hfill
\begin{subfigure}{0.3\textwidth}
        \centering
         \includegraphics[height=0.15\textheight,keepaspectratio]{Figures/drupalcombined/drupal_combined_tor_hiddenservices.pdf}
         %\caption{Struts CVE-207-5638}
         %\label{fig:drupal_allrocs}
\end{subfigure}
\caption{ROC curves for attack scripts for Drupal CVE-2018-7600}
%\label{fig:allrocs}
\end{figure*}

\begin{figure*}[h]
\centering
\begin{subfigure}{0.3\textwidth}
	\centering
	\includegraphics[height=0.15\textheight,keepaspectratio]{Figures/proftpdcombined/proftpd_combined_checkcontainer.pdf}
	%\caption{Drupal}
	%\label{fig:drupal_allrocs}
\end{subfigure}
\hfill
\begin{subfigure}{0.3\textwidth}
         \centering
         \includegraphics[height=0.15\textheight,keepaspectratio]{Figures/proftpdcombined/proftpd_combined_ecryptfs_creds.pdf}
         %\caption{ProFTPD}
         %\label{fig:proftpd_allrocs}
\end{subfigure}
\hfill
\begin{subfigure}{0.3\textwidth}
        \centering
         \includegraphics[height=0.15\textheight,keepaspectratio]{Figures/proftpdcombined/proftpd_combined_enum_configs.pdf}
         %\caption{Struts CVE-207-5638}
         %\label{fig:proftpd_allrocs}
\end{subfigure}

\smallskip
\begin{subfigure}{0.3\textwidth}
	\centering
	\includegraphics[height=0.15\textheight,keepaspectratio]{Figures/proftpdcombined/proftpd_combined_enum_network.pdf}
	%\caption{Drupal}
	%\label{fig:drupal_allrocs}
\end{subfigure}
\hfill
\begin{subfigure}{0.3\textwidth}
         \centering
         \includegraphics[height=0.15\textheight,keepaspectratio]{Figures/proftpdcombined/proftpd_combined_enum_protections.pdf}
         %\caption{ProFTPD}
         %\label{fig:proftpd_allrocs}
\end{subfigure}
\hfill
\begin{subfigure}{0.3\textwidth}
        \centering
         \includegraphics[height=0.15\textheight,keepaspectratio]{Figures/proftpdcombined/proftpd_combined_enum_psk.pdf}
         %\caption{Struts CVE-207-5638}
         %\label{fig:proftpd_allrocs}
\end{subfigure}

\smallskip
\begin{subfigure}{0.3\textwidth}
	\centering
	\includegraphics[height=0.15\textheight,keepaspectratio]{Figures/proftpdcombined/proftpd_combined_enum_system.pdf}
	%\caption{Drupal}
	%\label{fig:drupal_allrocs}
\end{subfigure}
\hfill
\begin{subfigure}{0.3\textwidth}
         \centering
         \includegraphics[height=0.15\textheight,keepaspectratio]{Figures/proftpdcombined/proftpd_combined_enum_users_history.pdf}
         %\caption{ProFTPD}
         %\label{fig:proftpd_allrocs}
\end{subfigure}
\hfill
\begin{subfigure}{0.3\textwidth}
        \centering
         \includegraphics[height=0.15\textheight,keepaspectratio]{Figures/proftpdcombined/proftpd_combined_enum_xchat.pdf}
         %\caption{Struts CVE-207-5638}
         %\label{fig:proftpd_allrocs}
\end{subfigure}

\smallskip
\begin{subfigure}{0.3\textwidth}
	\centering
	\includegraphics[height=0.15\textheight,keepaspectratio]{Figures/proftpdcombined/proftpd_combined_env.pdf}
	%\caption{Drupal}
	%\label{fig:drupal_allrocs}
\end{subfigure}
\hfill
\begin{subfigure}{0.3\textwidth}
         \centering
         \includegraphics[height=0.15\textheight,keepaspectratio]{Figures/proftpdcombined/proftpd_combined_gnome_commander_creds.pdf}
         %\caption{ProFTPD}
         %\label{fig:proftpd_allrocs}
\end{subfigure}
\hfill
\begin{subfigure}{0.3\textwidth}
        \centering
         \includegraphics[height=0.15\textheight,keepaspectratio]{Figures/proftpdcombined/proftpd_combined_hashdump.pdf}
         %\caption{Struts CVE-207-5638}
         %\label{fig:proftpd_allrocs}
\end{subfigure}

\smallskip
\begin{subfigure}{0.3\textwidth}
	\centering
	\includegraphics[height=0.15\textheight,keepaspectratio]{Figures/proftpdcombined/proftpd_combined_mount_cifs_creds.pdf}
	%\caption{Drupal}
	%\label{fig:drupal_allrocs}
\end{subfigure}
\hfill
\begin{subfigure}{0.3\textwidth}
         \centering
         \includegraphics[height=0.15\textheight,keepaspectratio]{Figures/proftpdcombined/proftpd_combined_pptpd_chap_secrets.pdf}
         %\caption{ProFTPD}
         %\label{fig:proftpd_allrocs}
\end{subfigure}
\hfill
\begin{subfigure}{0.3\textwidth}
        \centering
         \includegraphics[height=0.15\textheight,keepaspectratio]{Figures/proftpdcombined/proftpd_combined_tor_hiddenservices.pdf}
         %\caption{Struts CVE-207-5638}
         %\label{fig:proftpd_allrocs}
\end{subfigure}
\caption{ROC curves for attack scripts for ProFTPD CVE-2015-3306}
%\label{fig:allrocs}
\end{figure*}

\begin{figure*}[h]
\centering
\begin{subfigure}{0.3\textwidth}
	\centering
	\includegraphics[height=0.15\textheight,keepaspectratio]{Figures/wpajaxcombined/wpajaxloadmore_combined_checkcontainer.pdf}
	%\caption{Drupal}
	%\label{fig:drupal_allrocs}
\end{subfigure}
\hfill
\begin{subfigure}{0.3\textwidth}
         \centering
         \includegraphics[height=0.15\textheight,keepaspectratio]{Figures/wpajaxcombined/wpajaxloadmore_combined_ecryptfs_creds.pdf}
         %\caption{ProFTPD}
         %\label{fig:proftpd_allrocs}
\end{subfigure}
\hfill
\begin{subfigure}{0.3\textwidth}
        \centering
         \includegraphics[height=0.15\textheight,keepaspectratio]{Figures/wpajaxcombined/wpajaxloadmore_combined_enum_configs.pdf}
         %\caption{Struts CVE-207-5638}
         %\label{fig:wpajaxloadmore_allrocs}
\end{subfigure}

\smallskip
\begin{subfigure}{0.3\textwidth}
	\centering
	\includegraphics[height=0.15\textheight,keepaspectratio]{Figures/wpajaxcombined/wpajaxloadmore_combined_enum_network.pdf}
	%\caption{Drupal}
	%\label{fig:drupal_allrocs}
\end{subfigure}
\hfill
\begin{subfigure}{0.3\textwidth}
         \centering
         \includegraphics[height=0.15\textheight,keepaspectratio]{Figures/wpajaxcombined/wpajaxloadmore_combined_enum_protections.pdf}
         %\caption{ProFTPD}
         %\label{fig:proftpd_allrocs}
\end{subfigure}
\hfill
\begin{subfigure}{0.3\textwidth}
        \centering
         \includegraphics[height=0.15\textheight,keepaspectratio]{Figures/wpajaxcombined/wpajaxloadmore_combined_enum_psk.pdf}
         %\caption{Struts CVE-207-5638}
         %\label{fig:wpajaxloadmore_allrocs}
\end{subfigure}

\smallskip
\begin{subfigure}{0.3\textwidth}
	\centering
	\includegraphics[height=0.15\textheight,keepaspectratio]{Figures/wpajaxcombined/wpajaxloadmore_combined_enum_system.pdf}
	%\caption{Drupal}
	%\label{fig:drupal_allrocs}
\end{subfigure}
\hfill
\begin{subfigure}{0.3\textwidth}
         \centering
         \includegraphics[height=0.15\textheight,keepaspectratio]{Figures/wpajaxcombined/wpajaxloadmore_combined_enum_users_history.pdf}
         %\caption{ProFTPD}
         %\label{fig:proftpd_allrocs}
\end{subfigure}
\hfill
\begin{subfigure}{0.3\textwidth}
        \centering
         \includegraphics[height=0.15\textheight,keepaspectratio]{Figures/wpajaxcombined/wpajaxloadmore_combined_enum_xchat.pdf}
         %\caption{Struts CVE-207-5638}
         %\label{fig:wpajaxloadmore_allrocs}
\end{subfigure}

\smallskip
\begin{subfigure}{0.3\textwidth}
	\centering
	\includegraphics[height=0.15\textheight,keepaspectratio]{Figures/wpajaxcombined/wpajaxloadmore_combined_env.pdf}
	%\caption{Drupal}
	%\label{fig:drupal_allrocs}
\end{subfigure}
\hfill
\begin{subfigure}{0.3\textwidth}
         \centering
         \includegraphics[height=0.15\textheight,keepaspectratio]{Figures/wpajaxcombined/wpajaxloadmore_combined_gnome_commander_creds.pdf}
         %\caption{ProFTPD}
         %\label{fig:proftpd_allrocs}
\end{subfigure}
\hfill
\begin{subfigure}{0.3\textwidth}
        \centering
         \includegraphics[height=0.15\textheight,keepaspectratio]{Figures/wpajaxcombined/wpajaxloadmore_combined_hashdump.pdf}
         %\caption{Struts CVE-207-5638}
         %\label{fig:wpajaxloadmore_allrocs}
\end{subfigure}

\smallskip
\begin{subfigure}{0.3\textwidth}
	\centering
	\includegraphics[height=0.15\textheight,keepaspectratio]{Figures/wpajaxcombined/wpajaxloadmore_combined_mount_cifs_creds.pdf}
	%\caption{Drupal}
	%\label{fig:drupal_allrocs}
\end{subfigure}
\hfill
\begin{subfigure}{0.3\textwidth}
         \centering
         \includegraphics[height=0.15\textheight,keepaspectratio]{Figures/wpajaxcombined/wpajaxloadmore_combined_pptpd_chap_secrets.pdf}
         %\caption{ProFTPD}
         %\label{fig:proftpd_allrocs}
\end{subfigure}
\hfill
\begin{subfigure}{0.3\textwidth}
        \centering
         \includegraphics[height=0.15\textheight,keepaspectratio]{Figures/wpajaxcombined/wpajaxloadmore_combined_tor_hiddenservices.pdf}
         %\caption{Struts CVE-207-5638}
         %\label{fig:wpajaxloadmore_allrocs}
\end{subfigure}
\caption{ROC curves for attack scripts for WP Ajax Load More plugin}
%\label{fig:allrocs}
\end{figure*}

\begin{figure*}[h]
\centering
\begin{subfigure}{0.3\textwidth}
	\centering
	\includegraphics[height=0.15\textheight,keepaspectratio]{Figures/wpnmediacombined/wpnmedia_combined_checkcontainer.pdf}
	%\caption{Drupal}
	%\label{fig:drupal_allrocs}
\end{subfigure}
\hfill
\begin{subfigure}{0.3\textwidth}
         \centering
         \includegraphics[height=0.15\textheight,keepaspectratio]{Figures/wpnmediacombined/wpnmedia_combined_ecryptfs_creds.pdf}
         %\caption{ProFTPD}
         %\label{fig:proftpd_allrocs}
\end{subfigure}
\hfill
\begin{subfigure}{0.3\textwidth}
        \centering
         \includegraphics[height=0.15\textheight,keepaspectratio]{Figures/wpnmediacombined/wpnmedia_combined_enum_configs.pdf}
         %\caption{Struts CVE-207-5638}
         %\label{fig:wpnmedia_allrocs}
\end{subfigure}

\smallskip
\begin{subfigure}{0.3\textwidth}
	\centering
	\includegraphics[height=0.15\textheight,keepaspectratio]{Figures/wpnmediacombined/wpnmedia_combined_enum_network.pdf}
	%\caption{Drupal}
	%\label{fig:drupal_allrocs}
\end{subfigure}
\hfill
\begin{subfigure}{0.3\textwidth}
         \centering
         \includegraphics[height=0.15\textheight,keepaspectratio]{Figures/wpnmediacombined/wpnmedia_combined_enum_protections.pdf}
         %\caption{ProFTPD}
         %\label{fig:proftpd_allrocs}
\end{subfigure}
\hfill
\begin{subfigure}{0.3\textwidth}
        \centering
         \includegraphics[height=0.15\textheight,keepaspectratio]{Figures/wpnmediacombined/wpnmedia_combined_enum_psk.pdf}
         %\caption{Struts CVE-207-5638}
         %\label{fig:wpnmedia_allrocs}
\end{subfigure}

\smallskip
\begin{subfigure}{0.3\textwidth}
	\centering
	\includegraphics[height=0.15\textheight,keepaspectratio]{Figures/wpnmediacombined/wpnmedia_combined_enum_system.pdf}
	%\caption{Drupal}
	%\label{fig:drupal_allrocs}
\end{subfigure}
\hfill
\begin{subfigure}{0.3\textwidth}
         \centering
         \includegraphics[height=0.15\textheight,keepaspectratio]{Figures/wpnmediacombined/wpnmedia_combined_enum_users_history.pdf}
         %\caption{ProFTPD}
         %\label{fig:proftpd_allrocs}
\end{subfigure}
\hfill
\begin{subfigure}{0.3\textwidth}
        \centering
         \includegraphics[height=0.15\textheight,keepaspectratio]{Figures/wpnmediacombined/wpnmedia_combined_enum_xchat.pdf}
         %\caption{Struts CVE-207-5638}
         %\label{fig:wpnmedia_allrocs}
\end{subfigure}

\smallskip
\begin{subfigure}{0.3\textwidth}
	\centering
	\includegraphics[height=0.15\textheight,keepaspectratio]{Figures/wpnmediacombined/wpnmedia_combined_env.pdf}
	%\caption{Drupal}
	%\label{fig:drupal_allrocs}
\end{subfigure}
\hfill
\begin{subfigure}{0.3\textwidth}
         \centering
         \includegraphics[height=0.15\textheight,keepaspectratio]{Figures/wpnmediacombined/wpnmedia_combined_gnome_commander_creds.pdf}
         %\caption{ProFTPD}
         %\label{fig:proftpd_allrocs}
\end{subfigure}
\hfill
\begin{subfigure}{0.3\textwidth}
        \centering
         \includegraphics[height=0.15\textheight,keepaspectratio]{Figures/wpnmediacombined/wpnmedia_combined_hashdump.pdf}
         %\caption{Struts CVE-207-5638}
         %\label{fig:wpnmedia_allrocs}
\end{subfigure}

\smallskip
\begin{subfigure}{0.3\textwidth}
	\centering
	\includegraphics[height=0.15\textheight,keepaspectratio]{Figures/wpnmediacombined/wpnmedia_combined_mount_cifs_creds.pdf}
	%\caption{Drupal}
	%\label{fig:drupal_allrocs}
\end{subfigure}
\hfill
\begin{subfigure}{0.3\textwidth}
         \centering
         \includegraphics[height=0.15\textheight,keepaspectratio]{Figures/wpnmediacombined/wpnmedia_combined_pptpd_chap_secrets.pdf}
         %\caption{ProFTPD}
         %\label{fig:proftpd_allrocs}
\end{subfigure}
\hfill
\begin{subfigure}{0.3\textwidth}
        \centering
         \includegraphics[height=0.15\textheight,keepaspectratio]{Figures/wpnmediacombined/wpnmedia_combined_tor_hiddenservices.pdf}
         %\caption{Struts CVE-207-5638}
         %\label{fig:wpnmedia_allrocs}
\end{subfigure}
\caption{ROC curves for attack scripts for WP Nmedia Contact Form plugin}
%\label{fig:allrocs}
\end{figure*}

\begin{figure*}[h]
\centering
\begin{subfigure}{0.3\textwidth}
	\centering
	\includegraphics[height=0.15\textheight,keepaspectratio]{Figures/wpreflexcombined/wpreflex_combined_checkcontainer.pdf}
	%\caption{Drupal}
	%\label{fig:drupal_allrocs}
\end{subfigure}
\hfill
\begin{subfigure}{0.3\textwidth}
         \centering
         \includegraphics[height=0.15\textheight,keepaspectratio]{Figures/wpreflexcombined/wpreflex_combined_ecryptfs_creds.pdf}
         %\caption{ProFTPD}
         %\label{fig:proftpd_allrocs}
\end{subfigure}
\hfill
\begin{subfigure}{0.3\textwidth}
        \centering
         \includegraphics[height=0.15\textheight,keepaspectratio]{Figures/wpreflexcombined/wpreflex_combined_enum_configs.pdf}
         %\caption{Struts CVE-207-5638}
         %\label{fig:wpreflex_allrocs}
\end{subfigure}

\smallskip
\begin{subfigure}{0.3\textwidth}
	\centering
	\includegraphics[height=0.15\textheight,keepaspectratio]{Figures/wpreflexcombined/wpreflex_combined_enum_network.pdf}
	%\caption{Drupal}
	%\label{fig:drupal_allrocs}
\end{subfigure}
\hfill
\begin{subfigure}{0.3\textwidth}
         \centering
         \includegraphics[height=0.15\textheight,keepaspectratio]{Figures/wpreflexcombined/wpreflex_combined_enum_protections.pdf}
         %\caption{ProFTPD}
         %\label{fig:proftpd_allrocs}
\end{subfigure}
\hfill
\begin{subfigure}{0.3\textwidth}
        \centering
         \includegraphics[height=0.15\textheight,keepaspectratio]{Figures/wpreflexcombined/wpreflex_combined_enum_psk.pdf}
         %\caption{Struts CVE-207-5638}
         %\label{fig:wpreflex_allrocs}
\end{subfigure}

\smallskip
\begin{subfigure}{0.3\textwidth}
	\centering
	\includegraphics[height=0.15\textheight,keepaspectratio]{Figures/wpreflexcombined/wpreflex_combined_enum_system.pdf}
	%\caption{Drupal}
	%\label{fig:drupal_allrocs}
\end{subfigure}
\hfill
\begin{subfigure}{0.3\textwidth}
         \centering
         \includegraphics[height=0.15\textheight,keepaspectratio]{Figures/wpreflexcombined/wpreflex_combined_enum_users_history.pdf}
         %\caption{ProFTPD}
         %\label{fig:proftpd_allrocs}
\end{subfigure}
\hfill
\begin{subfigure}{0.3\textwidth}
        \centering
         \includegraphics[height=0.15\textheight,keepaspectratio]{Figures/wpreflexcombined/wpreflex_combined_enum_xchat.pdf}
         %\caption{Struts CVE-207-5638}
         %\label{fig:wpreflex_allrocs}
\end{subfigure}

\smallskip
\begin{subfigure}{0.3\textwidth}
	\centering
	\includegraphics[height=0.15\textheight,keepaspectratio]{Figures/wpreflexcombined/wpreflex_combined_env.pdf}
	%\caption{Drupal}
	%\label{fig:drupal_allrocs}
\end{subfigure}
\hfill
\begin{subfigure}{0.3\textwidth}
         \centering
         \includegraphics[height=0.15\textheight,keepaspectratio]{Figures/wpreflexcombined/wpreflex_combined_gnome_commander_creds.pdf}
         %\caption{ProFTPD}
         %\label{fig:proftpd_allrocs}
\end{subfigure}
\hfill
\begin{subfigure}{0.3\textwidth}
        \centering
         \includegraphics[height=0.15\textheight,keepaspectratio]{Figures/wpreflexcombined/wpreflex_combined_hashdump.pdf}
         %\caption{Struts CVE-207-5638}
         %\label{fig:wpreflex_allrocs}
\end{subfigure}

\smallskip
\begin{subfigure}{0.3\textwidth}
	\centering
	\includegraphics[height=0.15\textheight,keepaspectratio]{Figures/wpreflexcombined/wpreflex_combined_mount_cifs_creds.pdf}
	%\caption{Drupal}
	%\label{fig:drupal_allrocs}
\end{subfigure}
\hfill
\begin{subfigure}{0.3\textwidth}
         \centering
         \includegraphics[height=0.15\textheight,keepaspectratio]{Figures/wpreflexcombined/wpreflex_combined_pptpd_chap_secrets.pdf}
         %\caption{ProFTPD}
         %\label{fig:proftpd_allrocs}
\end{subfigure}
\hfill
\begin{subfigure}{0.3\textwidth}
        \centering
         \includegraphics[height=0.15\textheight,keepaspectratio]{Figures/wpreflexcombined/wpreflex_combined_tor_hiddenservices.pdf}
         %\caption{Struts CVE-207-5638}
         %\label{fig:wpreflex_allrocs}
\end{subfigure}
\caption{ROC curves for attack scripts for WP Reflex Gallery plugin CVE-2015-4133}
%\label{fig:allrocs}
\end{figure*}
